# Supplementary material for: DailyTalk: Spoken Dialogue Dataset for Conversational Text-to-Speech
Source: arXiv:2207.01063 source file (2023-03-13)
Supplement: Supplementary file 1 [file mos_criterion.tex]

\begin{table}[t]
\centering
\begin{subtable}{0.4\textwidth}
    \centering
    \begin{tabular}{c|c}
        \toprule
        Score & Explanation \\
        \midrule
        1 & Bad - Completely not human-like \\
        2 & Poor - Mostly not human-like \\
        3 & Equally human-like and not human-like \\
        4 & Good - Mostly human-like \\
        5 & Excellent - Completely human-like \\
        \bottomrule
    \end{tabular}
    \caption{MOS criteria}
\end{subtable}
\hfill
\begin{subtable}{0.4\textwidth}
    \centering
    \begin{tabular}{c|c}
        \toprule
        Score & Explanation (A vs. B) \\
        \midrule
        -3 & A is much better \\
        -2 & A is better \\
        -1 & A is slightly better \\
        0 & About the same \\
        1 & B is slightly better \\
        2 & B is better \\
        3 & B is much better \\
        \bottomrule
    \end{tabular}
    \caption{CMOS criteria}
\end{subtable}
    \caption{Criteria used for entire MOS test. We used widely-used 1 to 5 scale criteria for MOS test, and -3 to 3 scale used in \citet{guo2021conversational} for CMOS test.}
    \label{tab:mos_criterion}
\end{table}
