# Supplementary material for: DailyTalk: Spoken Dialogue Dataset for Conversational Text-to-Speech
Source: arXiv:2207.01063 source file (2023-03-13)
Supplement: Supplementary file 2 [file phoneme_list.tex]

\begin{table*}[t]
    \centering
    \begin{tabular}{l}
    \toprule
        \multicolumn{1}{c}{Phoneme List} \\
    \midrule
        "!", "'", ",", "-", ".", "?", "AA0", "AA1", "AA2", "AE0", "AE1", "AE2", "AH0", "AH1", "AH2", \\
        "AO0", "AO1", "AO2", "AW0", "AW1", "AW2", "AY0", "AY1", "AY2", "B", "CH", "D", "DH", \\
        "EH0", "EH1", "EH2", "ER0", "ER1", "ER2", "EY0", "EY1", "EY2", "F", "G", "HH", \\
        "IH0", "IH1", "IH2", "IY0", "IY1", "IY2", "JH", "K", "L", "M", "N", "NG", "OW0", "OW1", \\
        "OW2", "OY0", "OY1", "OY2", "P", "R", "S", "SH", "T", "TH", "UH0", "UH1", "UH2", "UW0", \\
        "UW1", "UW2", "V", "W", "Y", "Z", "ZH" \\
    \bottomrule
    \end{tabular}
    \caption{List of phonemes used in distribution (the X axis of figures in Figure~\ref{fig:phn_dt}). We follow CMUDict to represent each script as an aggregation of phonemes.}
    \label{tab:phoneme_list}
\end{table*}
