# Supplementary material for: DailyTalk: Spoken Dialogue Dataset for Conversational Text-to-Speech
Source: arXiv:2207.01063 source file (2023-03-13)
Supplement: Supplementary file 3 [file statistics_chr_dist.tex]

\begin{figure}
    \centering
    \subcaptionbox{Emotion Distribution}[.3\textwidth]{\includegraphics[width=.25\textwidth]{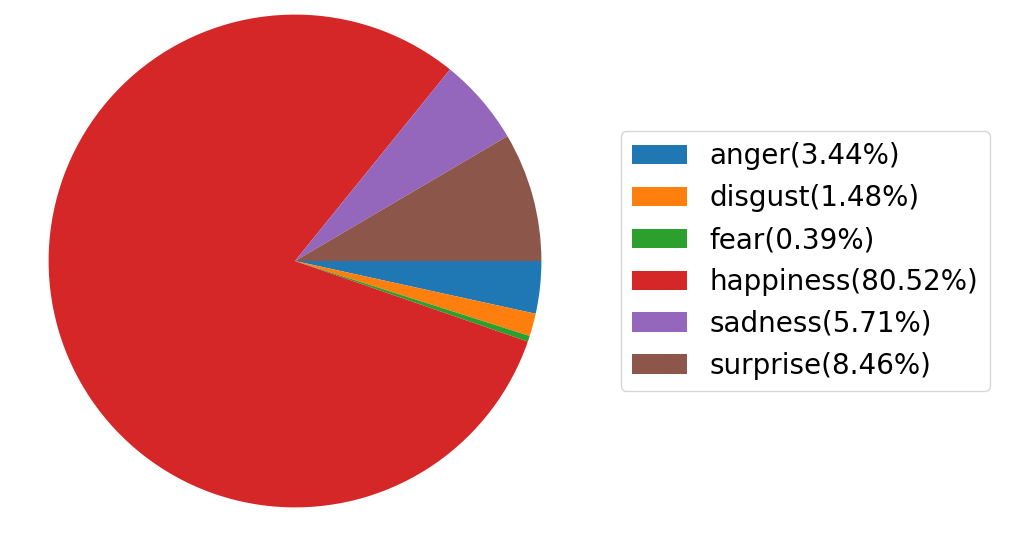}}
    \subcaptionbox{Topic Distribution}[.3\textwidth]{\includegraphics[width=.25\textwidth]{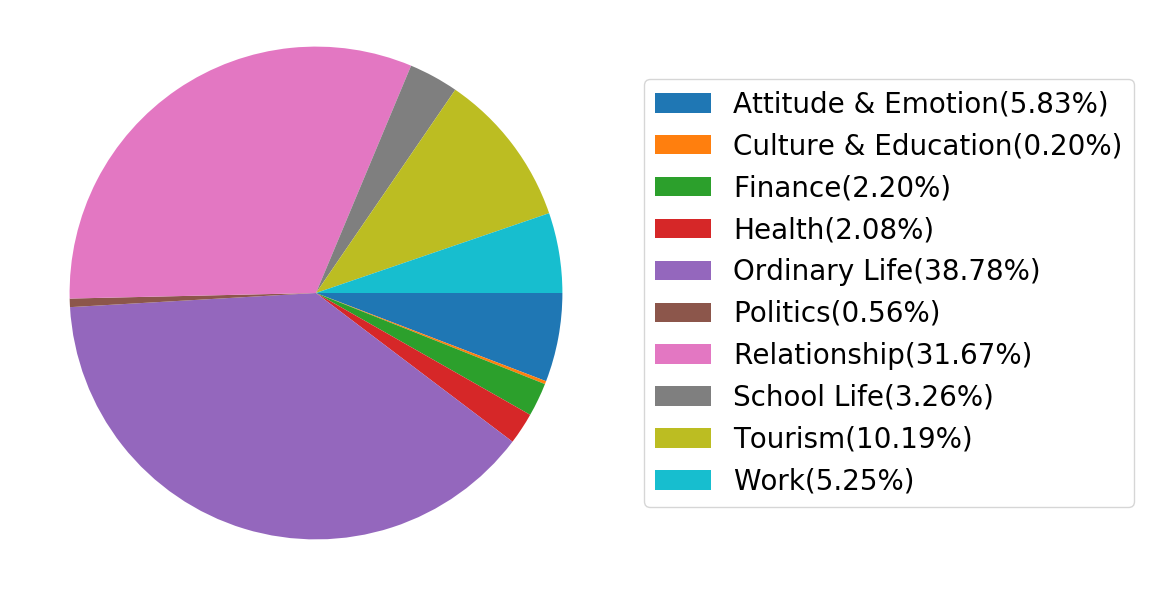}}
    \subcaptionbox{Dialogue Act Distribution}[.3\textwidth]{\includegraphics[width=.25\textwidth]{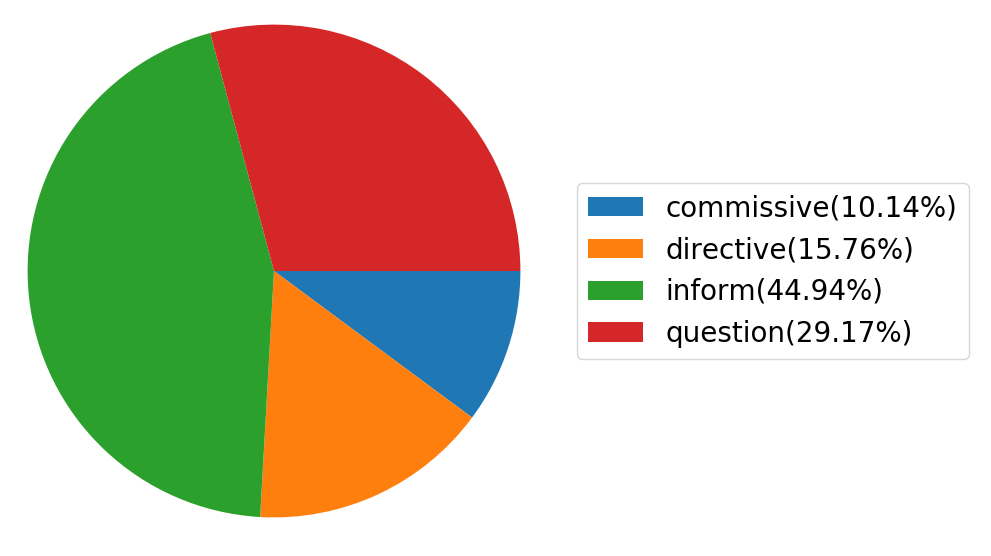}}
    
    \caption{Script-related distributions of \ours{}.}
    \label{fig:distributions_dt}
\end{figure}

% \begin{figure}
%     \begin{subfigure}{.3\textwidth}
%         \centering
%         \includegraphics[width=\textwidth]{images/emotion_distribution_total.png}
%         \caption{Emotion Distribution}
%     \end{subfigure}
%     \begin{subfigure}{.3\textwidth}
%         \centering
%         \includegraphics[width=\textwidth]{images/topic_distribution_total.png}
%         \caption{Topic Distribution}
%     \end{subfigure}
%     \begin{subfigure}{.3\textwidth}
%         \centering
%         \includegraphics[width=\textwidth]{images/dialogue_act_distribution_total.png}
%         \caption{Dialogue Act Distribution}
%     \end{subfigure}
%     \caption{Script-related distributions of \ours{}.}
%     \label{fig:distributions_dt}
% \end{figure}
