# Supplementary material for: DailyTalk: Spoken Dialogue Dataset for Conversational Text-to-Speech
Source: arXiv:2207.01063 source file (2023-03-13)
Supplement: Supplementary file 4 [file statistics_phn_dt.tex]

\begin{figure}[t]
    \centering
    \begin{subfigure}{.8\textwidth}
        \centering
        \includegraphics[width=\textwidth]{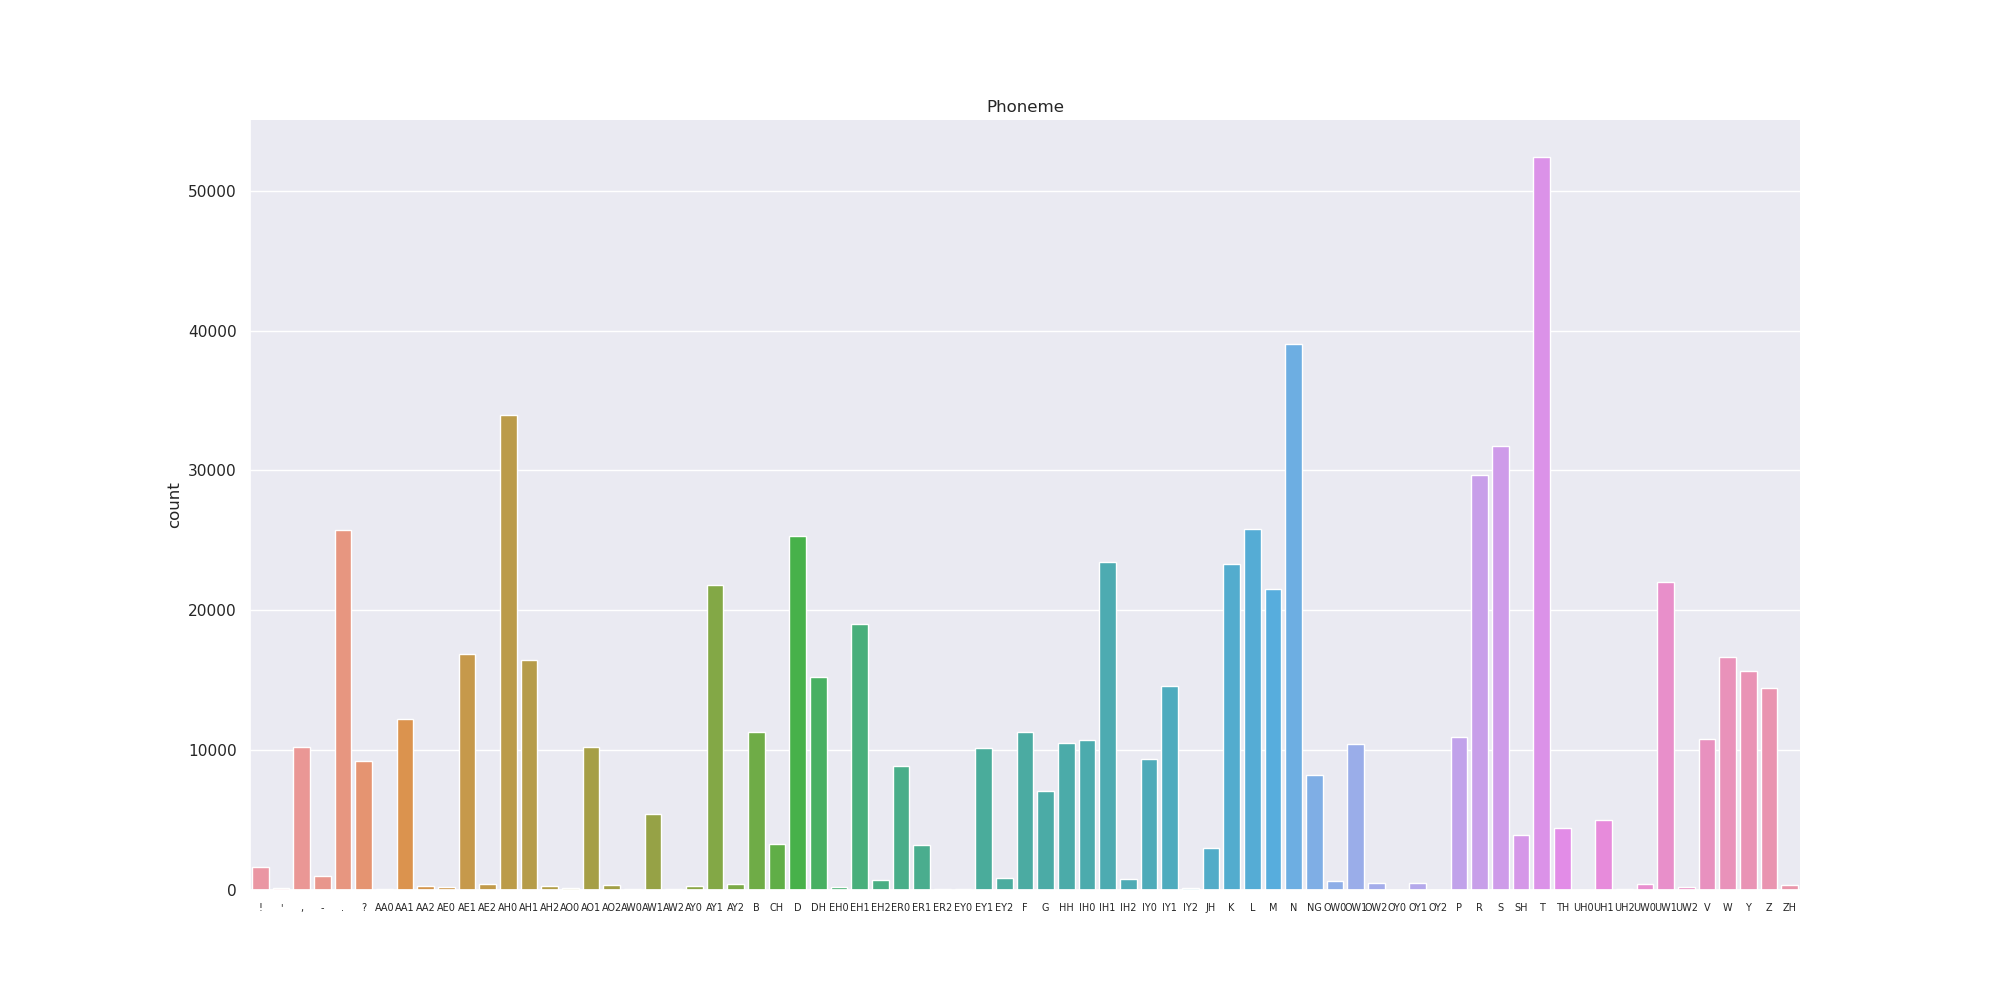}
        \caption{\ours{}}
    \end{subfigure}
    \begin{subfigure}{.4\textwidth}
        \centering
        \includegraphics[width=\textwidth]{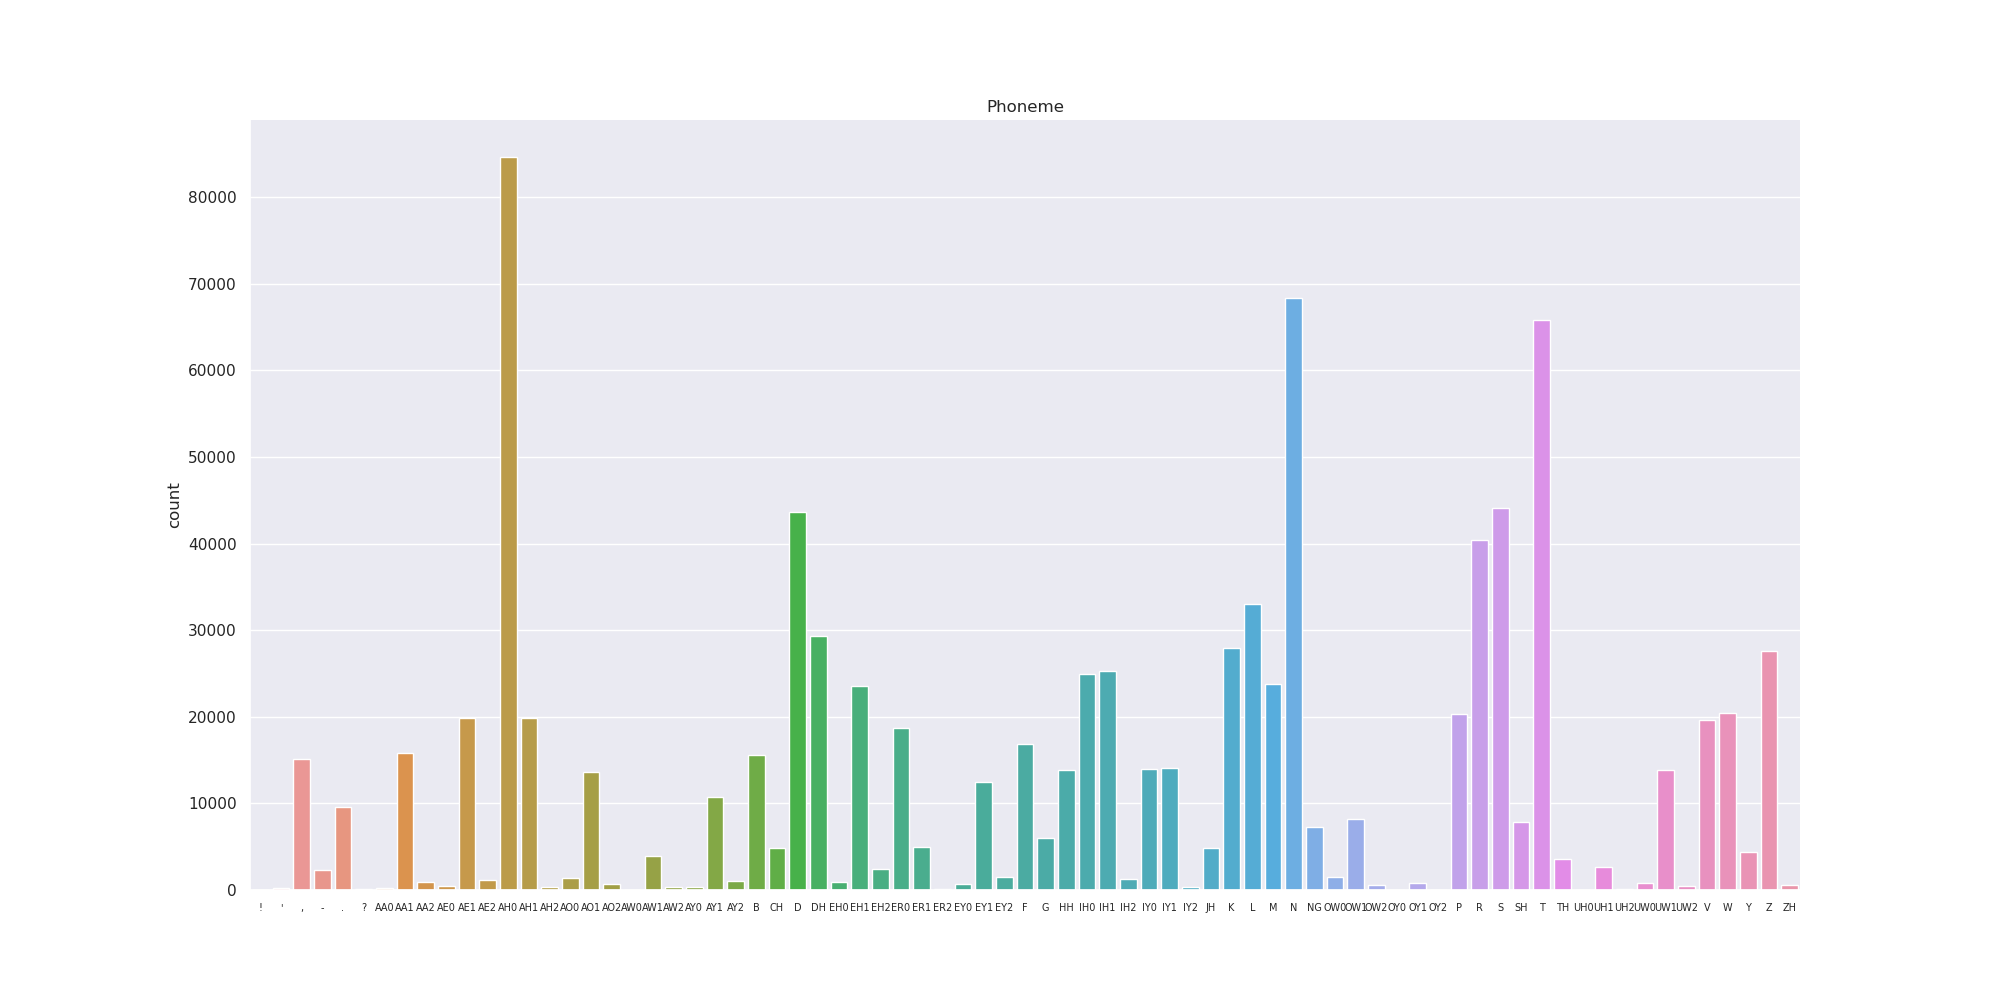}
        \caption{LJSpeech}
    \end{subfigure}
    \begin{subfigure}{.4\textwidth}
        \centering
        \includegraphics[width=\textwidth]{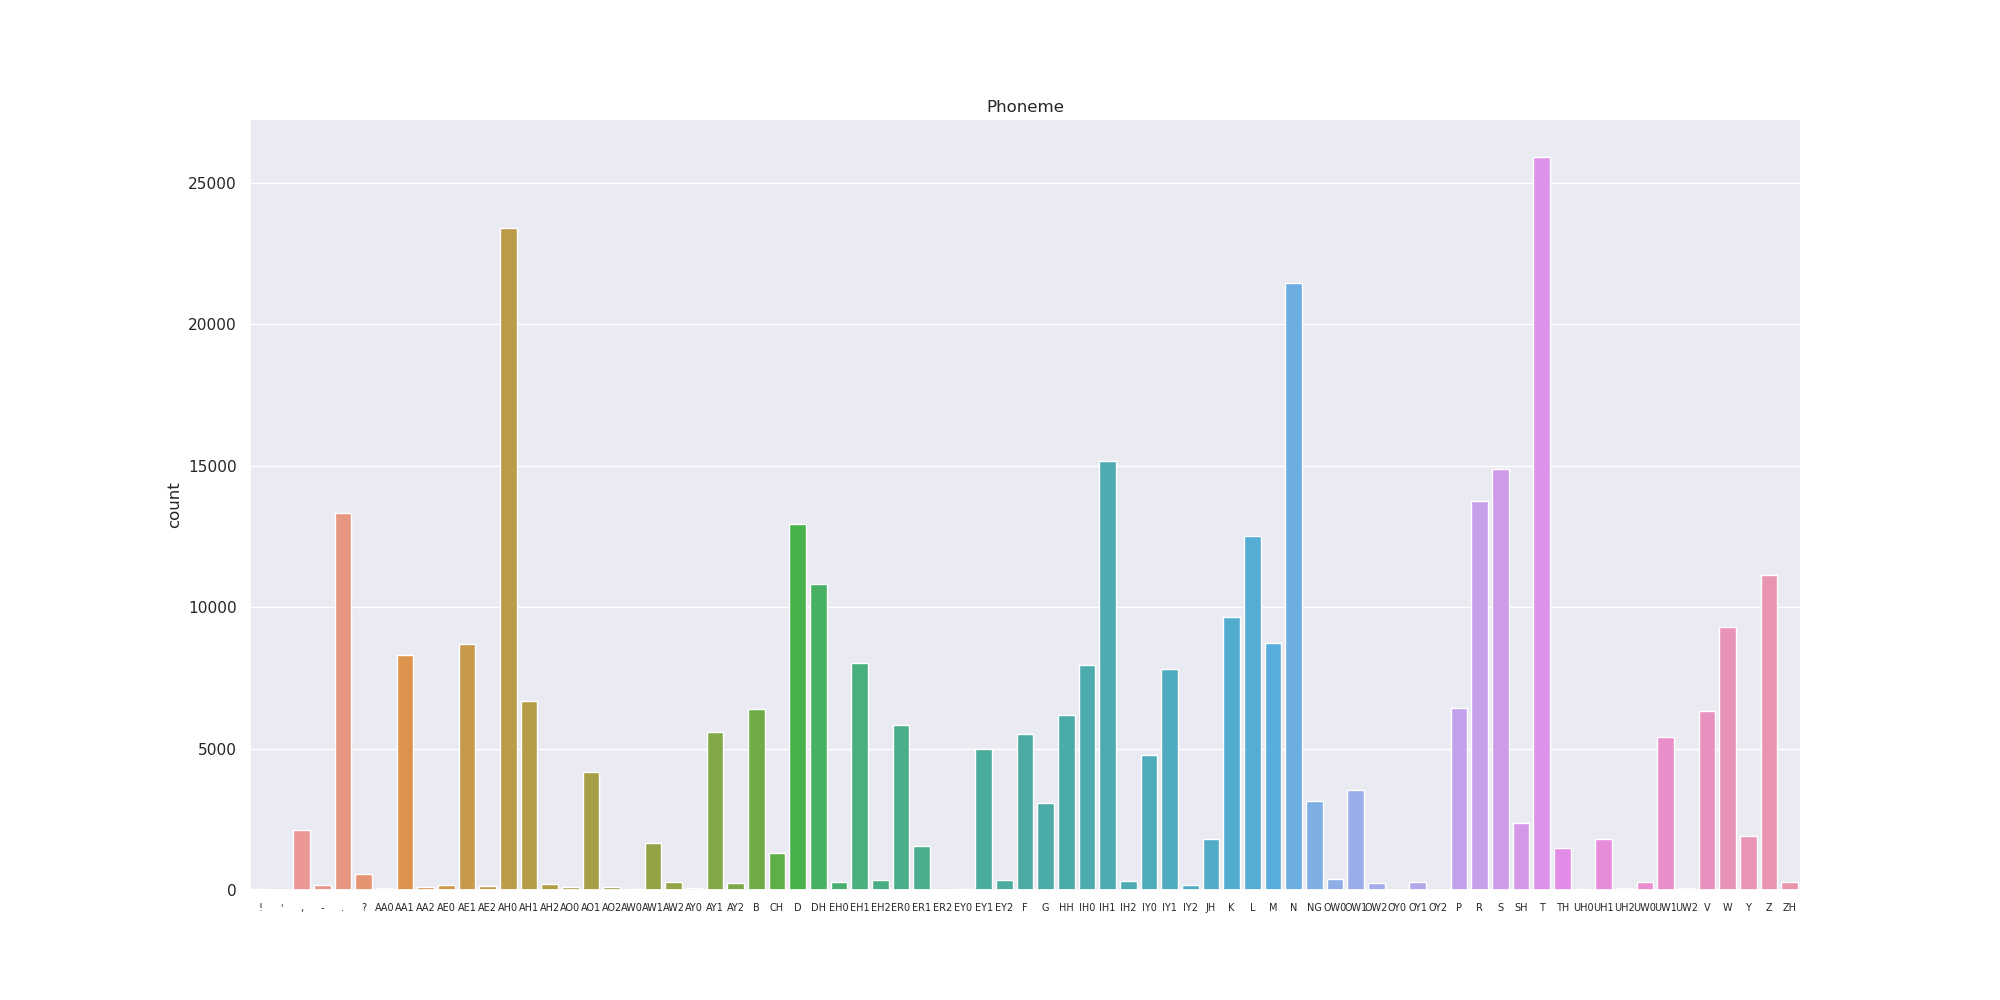}
        \caption{VCTK}
    \end{subfigure}
    \caption{Phoneme Distribution of \ours{}, LJSpeech, VCTK. Each bar represents occurrence of each phoneme. List of phonemes is from CMUDict. The X axis represents used phonemes in dataset, and the list of them is shown in Table~\ref{tab:phoneme_list}}
    \label{fig:phn_dt}
\end{figure}
