# Supplementary material for: DailyTalk: Spoken Dialogue Dataset for Conversational Text-to-Speech
Source: arXiv:2207.01063 source file (2023-03-13)
Supplement: Supplementary file 5 [file statistics_phn_others.tex]

\begin{figure}[h]
    \begin{subfigure}{.5\textwidth}
        \centering
        \includegraphics[width=\textwidth]{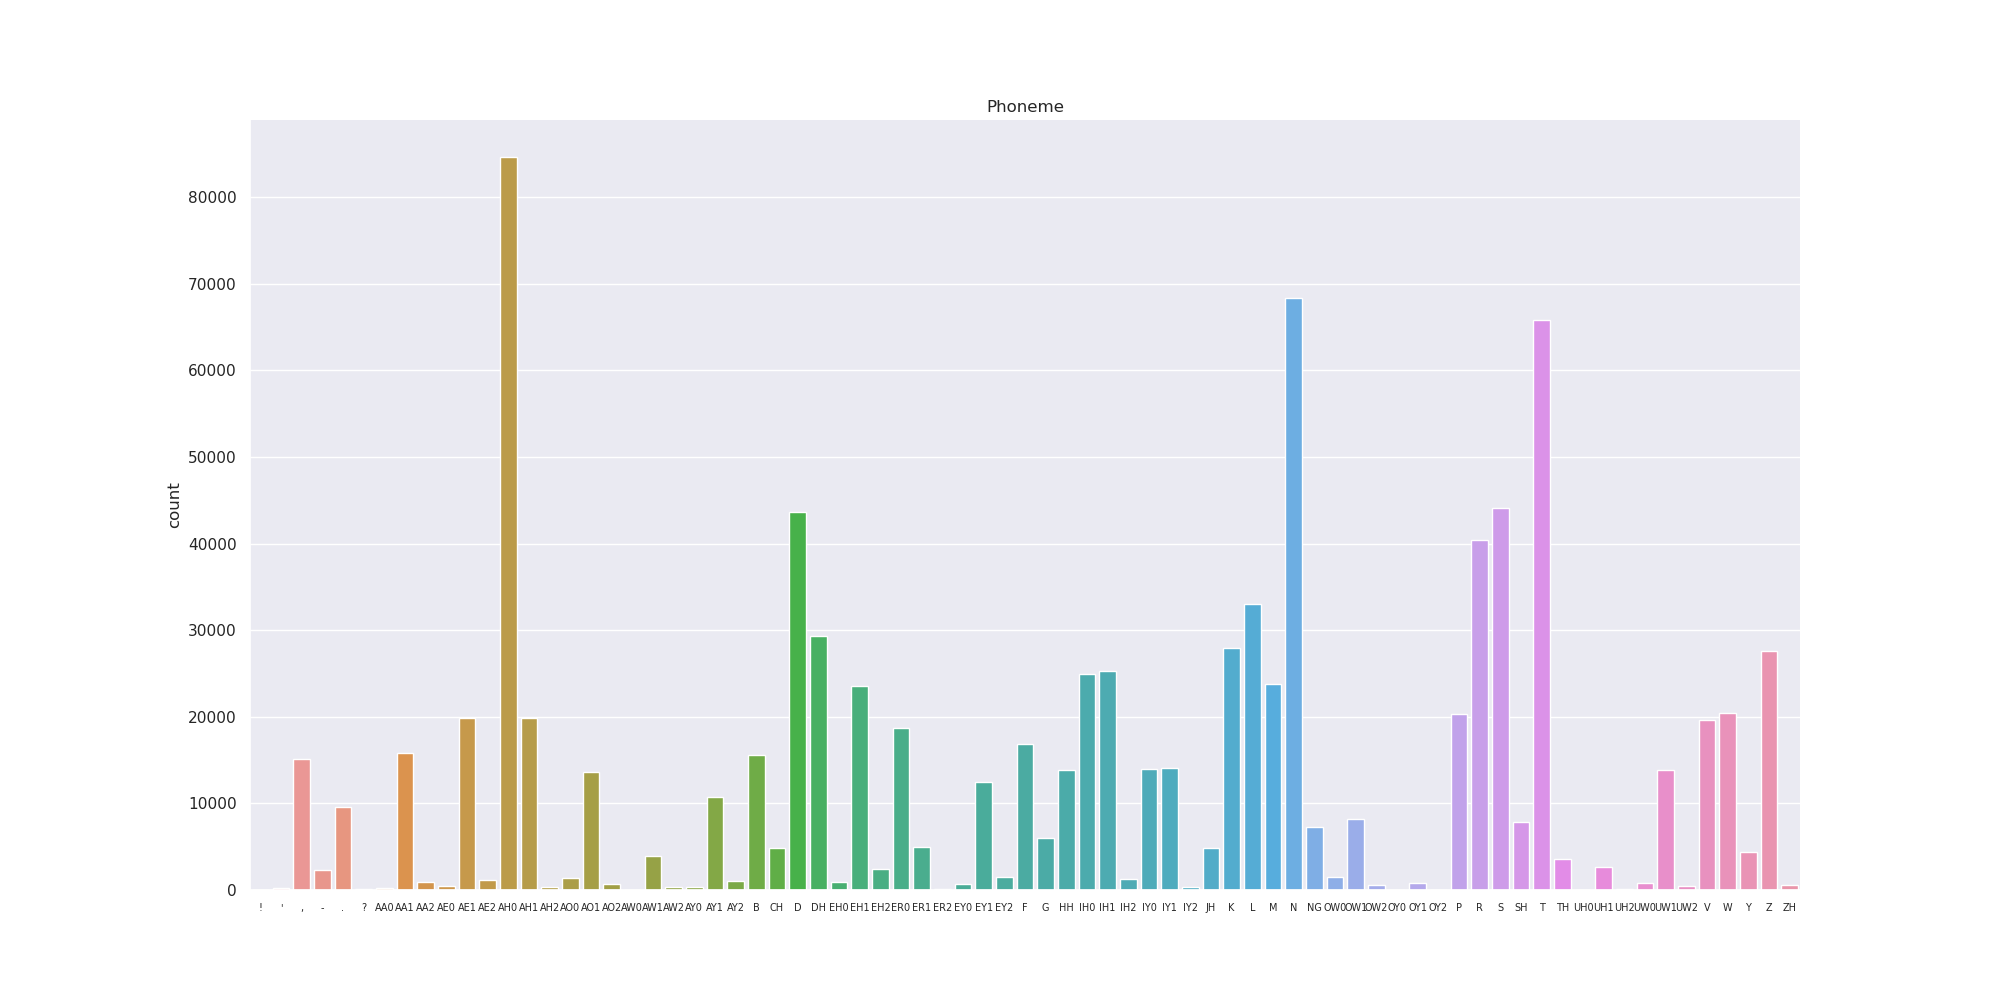}
        \caption{LJSpeech}
    \end{subfigure}
    \begin{subfigure}{.5\textwidth}
        \centering
        \includegraphics[width=\textwidth]{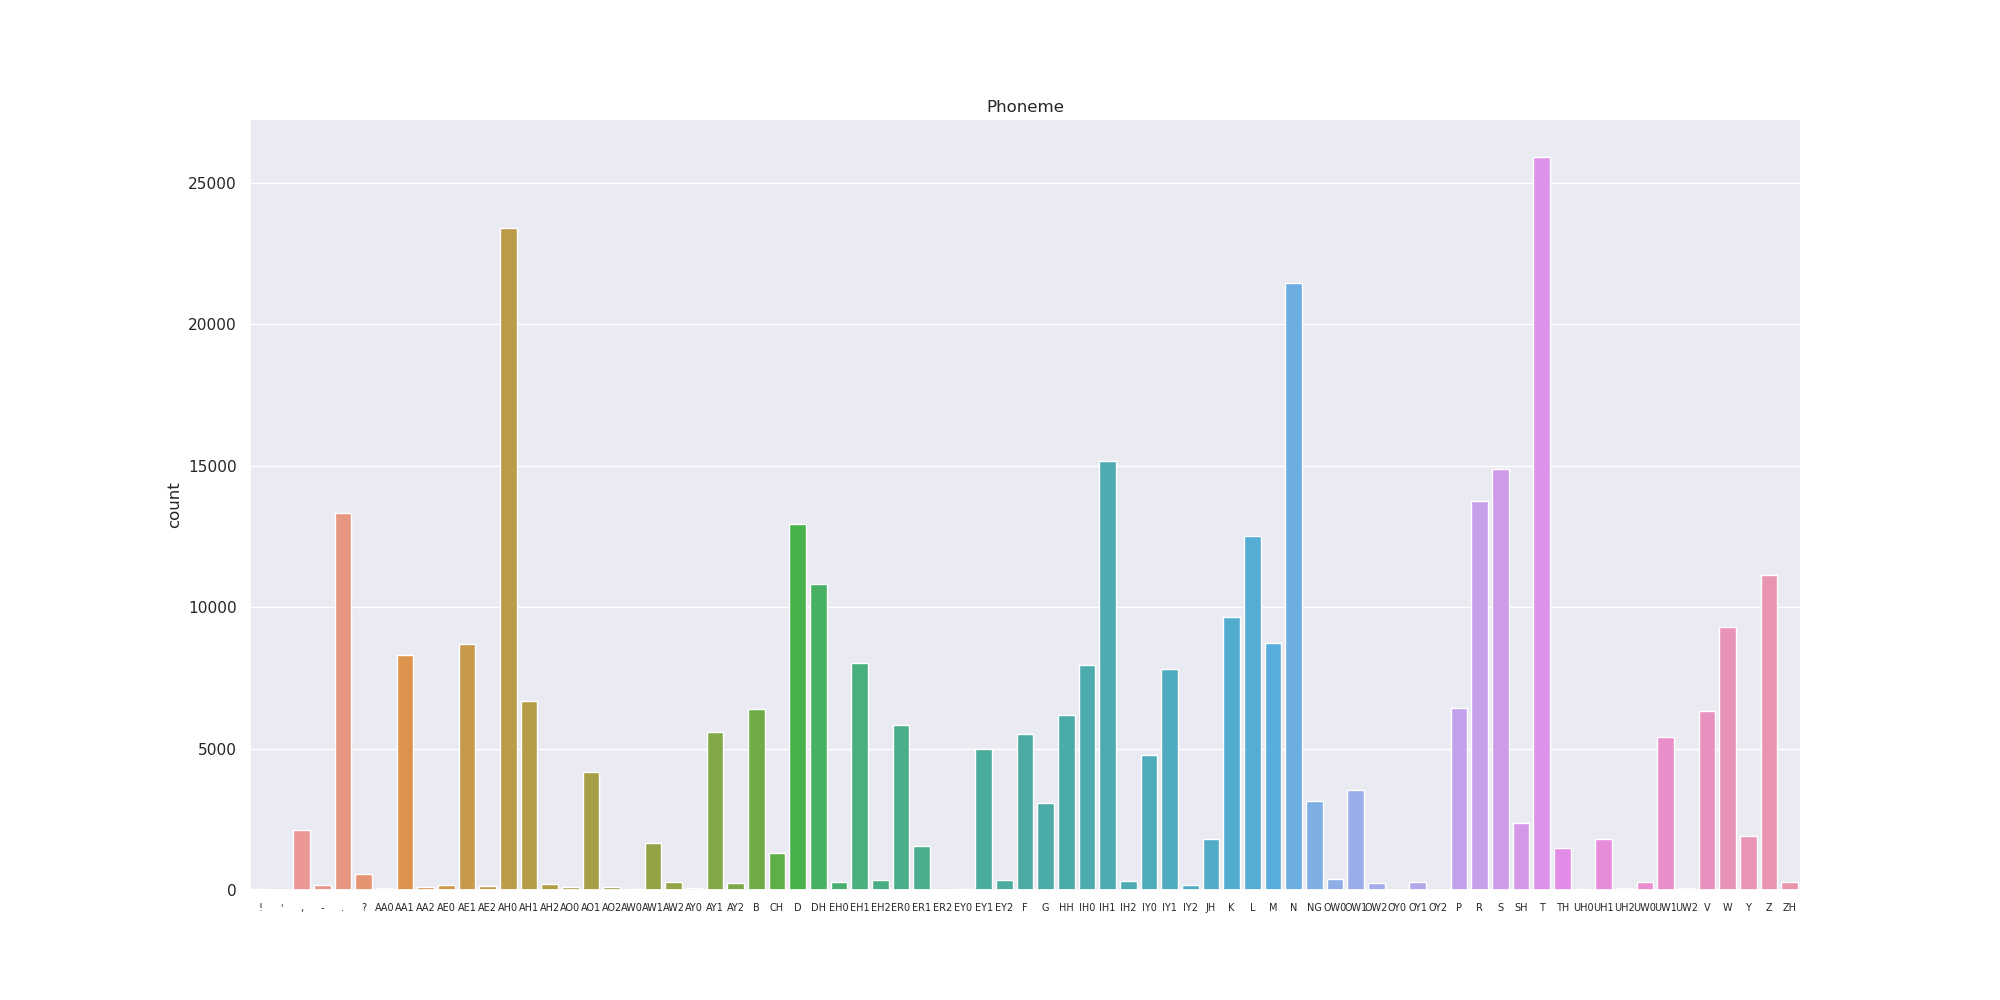}
        \caption{VCTK}
    \end{subfigure}
    \caption{Phoneme Distribution histogram of comparing datasets. We obtain distributions in the same method with \ours{}}
    \label{fig:distributions_others}
\end{figure}
