# Supplementary material for: DailyTalk: Spoken Dialogue Dataset for Conversational Text-to-Speech
Source: arXiv:2207.01063 source file (2023-03-13)
Supplement: Supplementary file 6 [file evaluation_sample.tex]

\begin{figure}[h]
    \centering
    \begin{subfigure}{.7\textwidth}
        \centering
        \includegraphics[width=\textwidth]{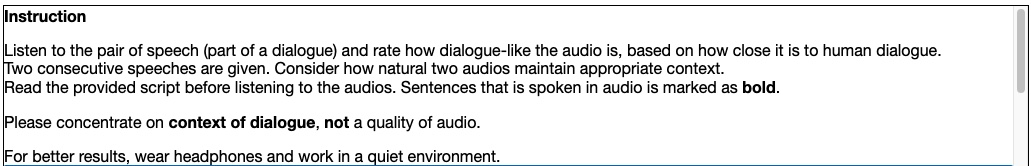}
        \caption{Evaluation Instruction}
    \end{subfigure}
    \begin{subfigure}{.7\textwidth}
        \centering
        \includegraphics[width=\textwidth]{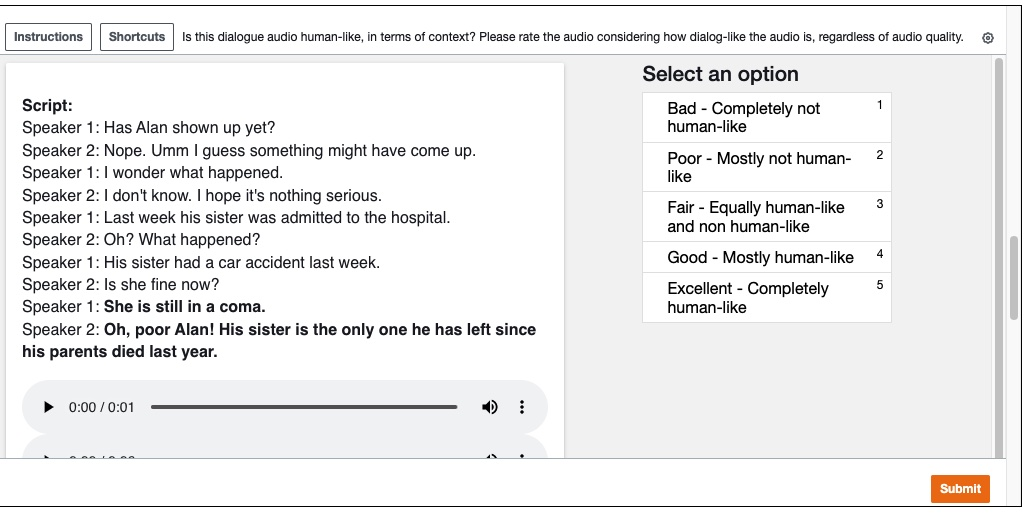}
        \caption{Evaluation Sample}
    \end{subfigure}
    \caption{Evaluation sample used in experiments. This sample is for Pairwise(synth pair) evaluation. We used same format of instruction and evaluation target for all human evaluations.}
    \label{fig:evaluation_sample}
\end{figure}
